# Supplementary material for: OMB-Py: Python Micro-Benchmarks for Evaluating Performance of MPI Libraries on HPC Systems
Source: arXiv:2110.10659 source file (2022-08-24)
Supplement: Supplementary file 1 [file appendix.tex]

\section{Artifact Description Appendix: OMB-Py}

%%%%%%%%%%%%%%%%%%%%%%%%%%%%%%%%%%%%%%%%%%%%%%%%%%%%%%%%%%%%%%%%%%%%%
\subsection{SUMMARY OF THE EXPERIMENTS REPORTED}

{\em 

The artifact contains the OMB-Py package that we have designed for this work.
OMB-Py is a micro-benchmarks package that is aimed to evaluate performance of MPI with the Python programming language using mpi4py for Python-MPI bindings. The package contains benchmarks for point-to-point and blocking collective MPI operations. In addition to CPU benchmarking, OMB-Py also supports GPU benchmarking by using GPU-aware arrays as  communication buffers. 

}

%%%%%%%%%%%%%%%%%%%%%%%%%%%%%%%%%%%%%%%%%%%%%%%%%%%%%%%%%%%%%%%%%%%%%
\subsection{Description}

\subsubsection{Check-list (artifact meta information)}

%{\em Fill in whatever is applicable with some informal keywords and remove the rest}

{\small
\begin{itemize}
  \item {\bf Algorithm: MPI operations benchmarks, distributed k-nearest neighbors, distributed hyperparameter optimization for k-means  }
  \item {\bf Program: Python code }
  \item {\bf Binary: .so library files for the CUDA aware MPI operations.}
  \item {\bf Dataset: Dota2 Games Results Data Set}
  \item {\bf Hardware: Intel Xeon Platinum 8280 and 8160 CPUs, Intel(R) Xeon(R) Gold 6132 CPU, and NVIDIA Tesla V100 GPUs}
  \item {\bf Output: Command line text output for different message sizes and measured metrics.}
  \item {\bf Experiment workflow: Download the wheel file, install using pip, run the
benchmarks on the required hardware.}
  \item {\bf Experiment customization: choose device to use (CPU or GPU), data buffer, message size range, number of main and warm-up iterations}
  \item {\bf Publicly available?: Yes }
\end{itemize}
}

\subsubsection{How software can be obtained (if available)}
In the future, we plan to release the software through project website and it will be 
downloadable without any restrictions. The ML benchmarks come as a separate package. \textit{Because the project website may violate 
the double-blind policy, this will be provided for the camera-ready version}.

\subsubsection{Hardware dependencies}
Intel Xeon Platinum 8280 and 8160 CPUs, Intel(R) Xeon(R) Gold 6132 CPU, and NVIDIA Tesla V100 GPUs were used for this study.

\subsubsection{Software dependencies}
Package requires mpi4py $>=$3.1.1, NumPy, CuPy, PyCUDA, Numba Python packages. 
These dependencies can be easily installed using the pip package manager.
We plan to distribute OMB-Py as a python wheel that can be easily installed using pip. 

In this study, we have used MVAPICH2 2.3.6 and MVAPICH2-GDR 2.3.6 communication runtime.
The steps to download and install MVAPICH2 and MVAPICH2\-GDR can be found here \textit{https://mvapich.cse.ohio-state.edu/downloads/}. 

We have used Miniconda package and environment management library to setup environment for experiments  on HPC systems. 

\subsubsection{Datasets}
\label{sec:dataset}
The Dota2 Games Results Data Set was used for the distributed k-nearest neighbors benchmark. A synthetic dataset is used for the distributed hyperparameter optimization for k-means benchmark.

%%%%%%%%%%%%%%%%%%%%%%%%%%%%%%%%%%%%%%%%%%%%%%%%%%%%%%%%%%%%%%%%%%%%%
\subsection{Installation}
We plan to release OMB-Py as a Python package that can be installed using pip package manager.
Download and install the wheel.

\vspace{1.0ex}

\noindent\fbox{
    \parbox{0.9\columnwidth}{%
\texttt{\$ wget http://xxx.xxx/OMB-Py.whl}

\texttt{\$ pip install OMB-Py.whl}
    }
}
\vspace{1.0ex}

%{\em Obligatory if the paper contains computational results.}

%%%%%%%%%%%%%%%%%%%%%%%%%%%%%%%%%%%%%%%%%%%%%%%%%%%%%%%%%%%%%%%%%%%%%
\subsection{Experiment workflow}

The following commands can be used to run the OMB-Py benchmarks on 2 CPUs.

\vspace{1.0ex}
\noindent\fbox{
    \parbox{0.9\columnwidth}{%
\texttt{\$ mpirun\_rsh --export-all -n 2 --hostfile hosts python OMB-Py.py 
--benchmark latency --mode CPU --buffer numpy}
}}

The following commands can be used to run the OMB-Py benchmarks on 2 GPUs.

\vspace{1.0ex}
\noindent\fbox{
    \parbox{0.9\columnwidth}{%
\texttt{\$ mpirun\_rsh --export-all -n 2 --hostfile hosts python OMB-Py.py 
--benchmark latency --mode CPU --buffer cupy}
}}

%%%%%%%%%%%%%%%%%%%%%%%%%%%%%%%%%%%%%%%%%%%%%%%%%%%%%%%%%%%%%%%%%%%%%
\vspace{1.0ex}
\subsection{Evaluation and expected result}

When running OMB-Py benchmarks, the results are generated as ASCII text to the standard I/O. The output will have a list of different message sizes in bytes and their measured metric: either latency in microseconds or bandwidth in MB/s depending on the tested benchmark. Each benchmark will run the MPI operation of interest for a number of iterations and calculate the overall average for all runs. Additionally, benchmarks will run some warm-up iterations before the actual test begins to report more accurate numbers.

%%%%%%%%%%%%%%%%%%%%%%%%%%%%%%%%%%%%%%%%%%%%%%%%%%%%%%%%%%%%%%%%%%%%%

\subsection{Experiment customization}
OMB-Py supports benchmarking for a series of MPI point-to-point and collective operations with a wide range of user options to run customizable tests.
\begin{itemize}
    \item --benchmark: available benchmarks are: latency, bw, bibw, mult\_lat, allgather, allreduce, alltoall, barrier, bcast, gather, reduce\_scatter, reduce, scatter, alltoallv, allgatherv, scatterv, and gatherv.
    \item --device: can choose either CPU or GPU devices to run the experiments on.
    \item --buffer: can choose from a list of Python objects to use as buffers. The list includes: bytearrays, Numpy, CuPy, PyCUDA, and Numba arrays.
    \item --lower-limit: defines lower limit for message sizes to report performance for.
    \item --upper-limit: defines upper limit for message sizes to report performance for.
    \item --iterations: defines number of times the tested MPI operation is executed. Reported performance numbers are the overall averages of all runs. weights and CSV file should be saved)
    \item --warm-up: defines the number of times to run the MPI operation before starting the actual test.
    
\end{itemize}

%%%%%%%%%%%%%%%%%%%%%%%%%%%%%%%%%%%%%%%%%%%%%%%%%%%%%%%%%%%%%%%%%%%%%
